# Supplementary material for: Hardware-Assisted Virtualization of Neural Processing Units for Cloud Platforms
Source: arXiv:2408.04104 source file (2024-09-13)
Supplement: Supplementary file 1 [file appendix.tex]

% \pagebreak

% \newpage
\begin{figure*}[t]
    \centering
    \includegraphics[width=\linewidth]{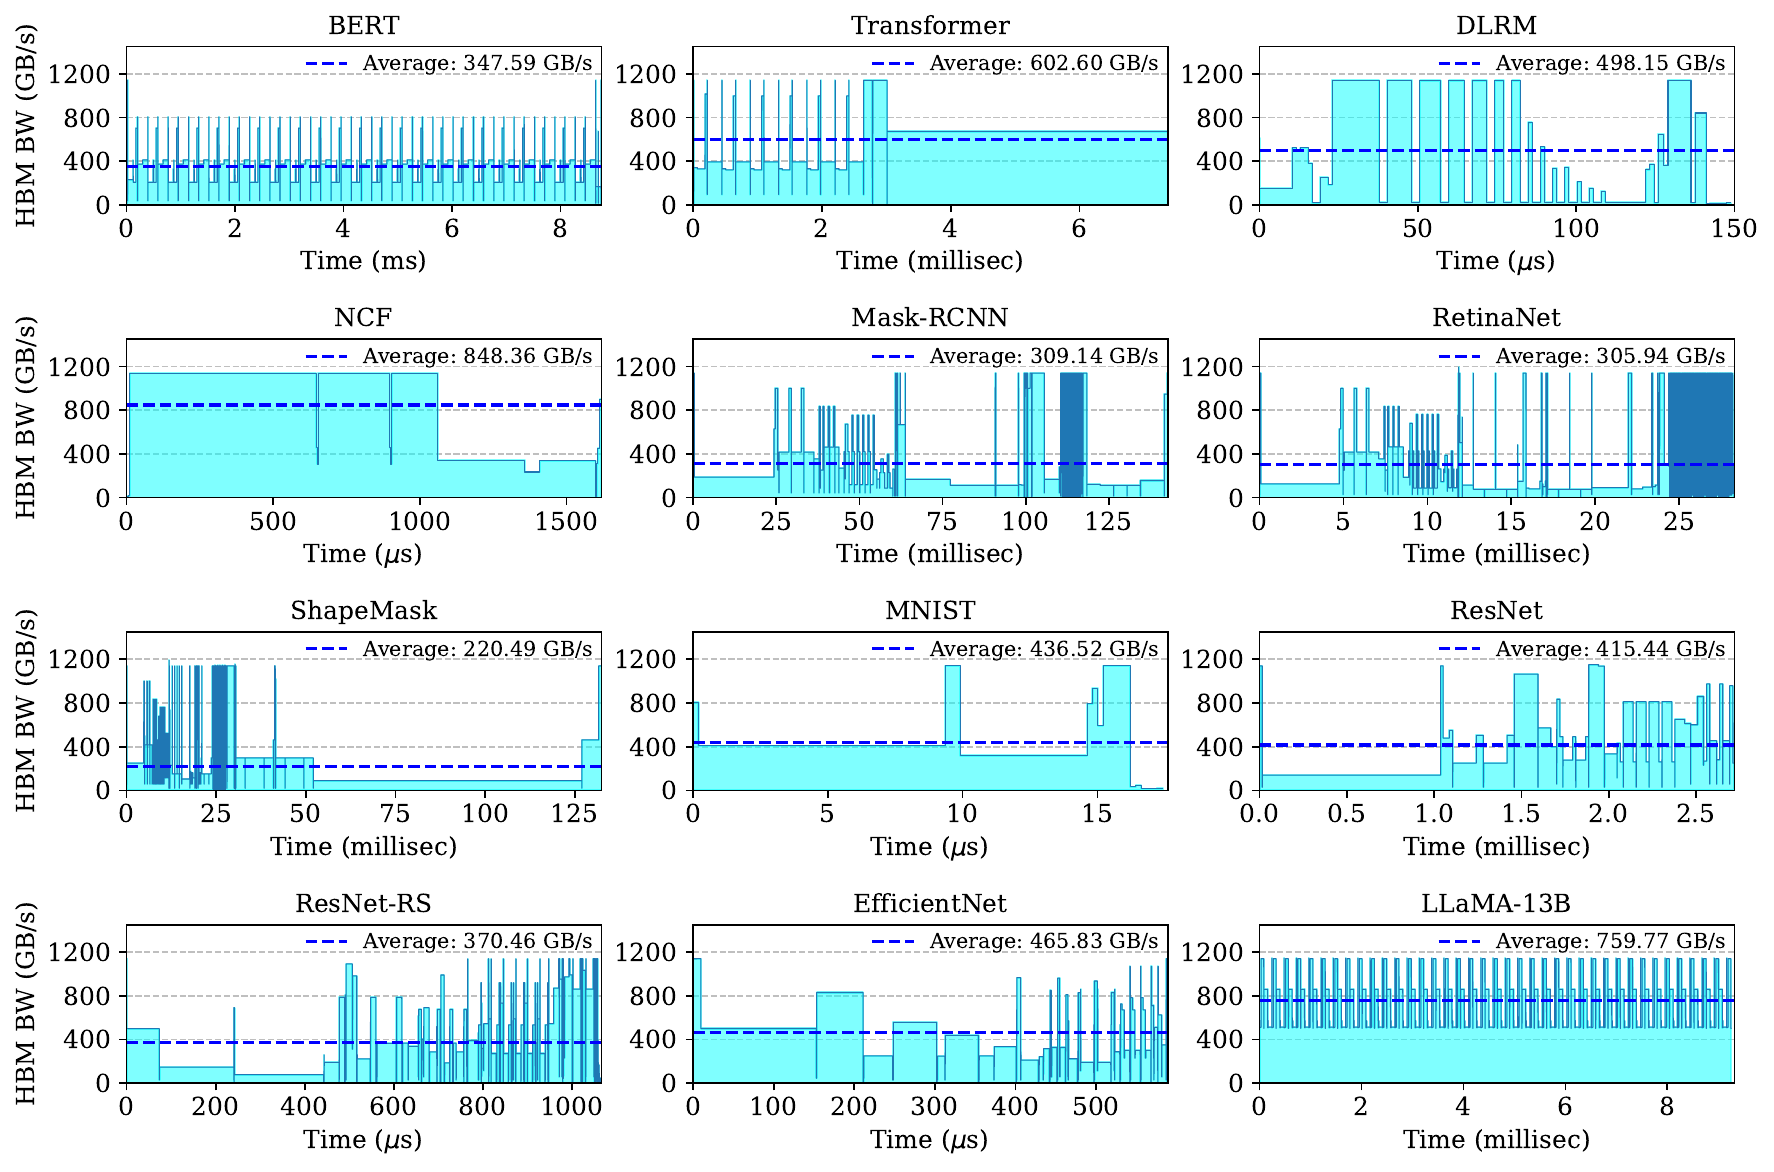}
    \caption{Memory bandwidth utilization of different ML inferences (batch size is 8).}
    \label{fig:hb_bw_vs_time_all}
\end{figure*}

\appendix

\section{Memory Bandwidth Demands of DNN Models}
\label{sec:mem_bw_all}

Following the experiment settings in \mbox{\S\ref{sec:npu_util_study}},
we plot the memory bandwidth utilization of various DNN models on a TPUv4 core in \mbox{\Cref{fig:hb_bw_vs_time_all}}. 
These models include popular DNN models used in machine learning services and a recent large language model (LLM) -- LLaMA-13B.
For many DNN models, their operators do not reach the peak memory bandwidth (1.2TB/s on a TPUv4 chip). 
The memory bandwidth requirement of a DNN model depends on both the model architecture and the model size.
For example, convolutional neural networks (CNNs) like ResNet and ShapeMask require less bandwidth than recommendation models (e.g., DLRM and NCF) 
and transformer-based models (e.g., BERT, Transformer, and LLaMA-13B).
For the same model architecture (e.g., both Transformer and LLaMA-13B have the same auto-regressive decoder-based architecture), 
a larger model (e.g., LLaMA-13B has 26GB weights and Transformer has 1.4GB weights) typically implies a higher memory bandwidth requirement, 
since it needs to read more weights from the HBM.
